# Supplementary material for: Majorana Spin Current Generation by Dynamic Strain
Source: arXiv:2301.03937 source file (2023-01-11)
Supplement: Supplementary file 1 [file Supplemental__Material.pdf]

# Supplemental Material: Majorana Spin Current Generation by Dynamic Strain

Yuki Yamazaki,[1] Takumi Funato,[2,3] and Ai Yamakage[1]

[1]*Department of Physics, Nagoya University, Nagoya 464-8602, Japan*

[2]*Center for Spintronics Research Network, Keio University, Yokohama 223-8522, Japan*

[3]*Kavli Institute for Theoretical Sciences, University of Chinese Academy of Sciences, Beijing, 100190, China*

(Dated: January 11, 2023)

## CONTENTS

I. Effective Hamiltonian on the (001) surface of antiperovskite 1
   A. Symmetry operation 1
   B. Hamiltonian 2
   C. Spin 3

II. Spin current induced by dynamic strain 3
   A. Spin current 4
   B. dynamic strain 4
   C. Calculation of $K^{(1)}_{ij}$ in the case of $M_z = 0$ 6
   D. Calculation of $K^{(1)}_{ij}$ in the case of $M_z \neq 0$ 7
   E. Calculation of $K_{11}(\omega)$ and $K_{12}(\omega)$ from Lehmann representation in the case of $M_z \neq 0$ 8
      1. $K_{11}(\omega)$ 8
      2. $K_{12}(\omega)$ 10

References 11

## I. EFFECTIVE HAMILTONIAN ON THE (001) SURFACE OF ANTIPEROVSKITE

By applying a general theory for MKPs proposed in the references [1, 2], we derive an effective Hamiltonian for double Majorana Kramers pairs (MKPs) emerging on the surface of a superconducting antiperovskite $Sr_3SnO$. Antiperovskites have the space group symmetry $Pm\bar{3}m$ (No. 221) [3, 4] and the corresponding point group (PG) $O_h$. The (001) surface has $p4m$ wallpaper group (WG) and $C_{4v}$ PG symmetry. It has been revealed that the $A_{1u}$ pairing in the bulk can induce double MKPs protected only by $C_{4z}$ rotational symmetry, on the $\bar{\Gamma}$ point in the surface Brillouin zone projected onto the (001) surface [5].

The double MKPs are spanned in the basis of zero-energy states of the Bogoliubov-de Gennes equation, $H_{\mathrm{BdG}}(k_x = 0, k_y = 0, z)\psi = 0$, in the semi-infinite space $z \leq 0$ on the $\bar{\Gamma}$ point, which is given by a double-valued, four-dimensional, and time-reversal-invariant representation of the little group of the $\bar{\Gamma}$ point. The representation that reproduces double MKPs on the (001) surface of $Sr_3SnO$ is given by $\bar{\Gamma}_6 \oplus \bar{\Gamma}_7$ [6, 7] since we consider that there only exists the finite magnetic winding number defined by $C_{4z}$ rotational symmetry [2, 5].

### A. Symmetry operation

The $\bar{\Gamma}_6 \oplus \bar{\Gamma}_7$ representation of the generators of the little group of $p4m$ is given by [6]

$$D_{\{C_{4z}|\mathbf{0}\}} = \begin{pmatrix} e^{i3\pi/4} & 0 & 0 & 0 \\ 0 & e^{-i3\pi/4} & 0 & 0 \\ 0 & 0 & e^{-i\pi/4} & 0 \\ 0 & 0 & 0 & e^{i\pi/4} \end{pmatrix} = \frac{-1}{\sqrt{2}}(s_0\tau_3 - is_3\tau_3), \tag{S.1}$$

$$D_{\{\sigma(xz)|\mathbf{0}\}} = \begin{pmatrix} 0 & e^{-i\pi/4} & 0 & 0 \\ e^{-i3\pi/4} & 0 & 0 & 0 \\ 0 & 0 & 0 & e^{i3\pi/4} \\ 0 & 0 & e^{i\pi/4} & 0 \end{pmatrix} = \frac{i}{\sqrt{2}}(s_2\tau_3 - s_1\tau_3). \tag{S.2}$$

TABLE I. Irreducible decomposition of the matrices, momentum, strain, and spin current in the $p4m$ model for the $A_{1u}$ superconducting pair potential in the bulk. Matrix is transformed by $g$ as $\eta \to D_g^\dagger \eta D_g$. $(\eta_i, \eta_j)$ denotes $(\eta_i, \eta_j) \to (-\eta_j, \eta_i)$ by transformation of $C_{4z}$ and $(\eta_i, \eta_j) \to (-\eta_i, \eta_j)$ by transformation of $\sigma(xz)$. Electric/magnetic and PHS denote time-reversal even/odd and particle-hole symmetry, respectively. $u_{ij}(\boldsymbol{x}) = \partial_i u_j(\boldsymbol{x})$ with $\boldsymbol{u}$ the displacement field. $j_i^\alpha$ denotes spin $\sigma^\alpha/2$ current along the $i$th direction.

| IR | electric w/ PHS | electric w/o PHS | magnetic w/ PHS | magnetic w/o PHS | momentum | Strain | Spin current |
|---|---|---|---|---|---|---|---|
| $A_1$ | | $s_0\tau_0, s_0\tau_3$ | | | $k_x^2 + k_y^2$ | $u_{xx} + u_{yy}$ | $j_y^x - j_x^y$ |
| $A_2$ | | | $s_3\tau_0, s_3\tau_3$ | | | $u_{xy} - u_{yx}$ | $j_x^x + j_y^y$ |
| $B_1$ | $s_3\tau_1$ | | | $s_3\tau_2$ | $k_x^2 - k_y^2$ | $u_{xx} - u_{yy}$ | $j_y^x + j_x^y$ |
| $B_2$ | $s_0\tau_2$ | | | $s_0\tau_1$ | $k_x k_y$ | $u_{xy} + u_{yx}$ | $j_x^x - j_y^y$ |
| $E$ | | $(\eta_7, \eta_8)$ | $(\eta_5, \eta_6)$ | $(\eta_1, \eta_2), (\eta_3, \eta_4)$ | $(k_x, k_y)$ | $(u_{xz}, u_{yz})$ | $(j_y^z, -j_x^z)$ |

The representation of chiral operator $\Gamma$ satisfies $\Gamma D_g = \chi_g D_g \Gamma$ [1], where $\chi_g$ denotes the character of representation to which the pair potential belongs. In the present case, we have assumed the pair potential to be $A_{1u}$ representation of $O_h$ in bulk and $A_2$ representation of $C_{4v}$ in the (001) surface. Therefore, $\chi_{C_{4z}} = 1$ and $\chi_{\sigma(xz)} = -1$. One finds that the following representation satisfies the condition.

$$\Gamma = \begin{pmatrix} 1 & 0 & 0 & 0 \\ 0 & -1 & 0 & 0 \\ 0 & 0 & -1 & 0 \\ 0 & 0 & 0 & 1 \end{pmatrix} = s_3\tau_3. \tag{S.3}$$

Note that the other possible representation is $\Gamma = s_3\tau_0$, which is rejected due to the contradiction with the topological invariants of $Sr_3SnO$ [2]. Time-reversal operator $\Theta$ is represented by $\Theta = s_2\tau_3 K$. Particle-hole transform is given by $C = i\Gamma\Theta$

$$C = \begin{pmatrix} 0 & 1 & 0 & 0 \\ 1 & 0 & 0 & 0 \\ 0 & 0 & 0 & 1 \\ 0 & 0 & 1 & 0 \end{pmatrix} K = s_1\tau_0 K. \tag{S.4}$$

From the above representations, one can derive the irreducible decomposition of the matrices $s_\mu\tau_\nu$'s, as summarized in Table I.

### B. Hamiltonian

The transformation of the Hamiltonian $H(\boldsymbol{k})$ by $g$ as

$$D_g H(\boldsymbol{k}) D_g^\dagger = H(g\boldsymbol{k}), \tag{S.5}$$

where a momentum $\boldsymbol{k}$ is transformed to $g\boldsymbol{k}$ under the action of $g$, i.e., $C_4\boldsymbol{k} = (-k_y, k_x)$ and $\sigma(xz)\boldsymbol{k} = (k_x, -k_y)$. The totally symmetric representations can appear in the Hamiltonian. Therefore we get

$$\begin{aligned} \hat{H} &= \frac{1}{2}\sum_{\boldsymbol{k}} \hat{\psi}_{\boldsymbol{k}}^\dagger H(\boldsymbol{k}) \hat{\psi}_{\boldsymbol{k}}, \\ H(\boldsymbol{k}) &= v_1(\eta_1 k_y - \eta_2 k_x) + v_2(\eta_3 k_y - \eta_4 k_x) - M_z \sigma_z, \end{aligned} \tag{S.6}$$

where $\hat{\psi}_{\boldsymbol{k}}^\dagger = (\hat{\psi}_{1\boldsymbol{k}}^\dagger, \hat{\psi}_{2\boldsymbol{k}}^\dagger, \hat{\psi}_{3\boldsymbol{k}}^\dagger, \hat{\psi}_{4\boldsymbol{k}}^\dagger)$ and $\hat{\psi}_{\boldsymbol{k}} = {}^t(\hat{\psi}_{1\boldsymbol{k}}, ..., \hat{\psi}_{4\boldsymbol{k}})$ are the Majorana creation/annihilation operators, which satisfy $\hat{\psi}_{1\boldsymbol{k}}^\dagger = \hat{\psi}_{2-\boldsymbol{k}}$ and $\hat{\psi}_{3\boldsymbol{k}}^\dagger = \hat{\psi}_{4-\boldsymbol{k}}$ to be consistent with PHS Eq. (S.4), $CH(\boldsymbol{k})C^{-1} = -H(-\boldsymbol{k})$. The anticommutation relation for the MKPs is given by

$$\left\{\hat{\psi}_{i\boldsymbol{k}}, \hat{\psi}_{j\boldsymbol{k}'}^\dagger\right\} = \delta_{ij}\delta_{\boldsymbol{k}\boldsymbol{k}'}, \quad \left\{\hat{\psi}_{i\boldsymbol{k}}, \hat{\psi}_{j\boldsymbol{k}'}\right\} = (s_1\tau_0)_{ij}\delta_{\boldsymbol{k},-\boldsymbol{k}'}. \tag{S.7}$$

Here is the diagonalization of the Hamiltonian. The Hamiltonian matrix $H(\boldsymbol{k})$ is decomposed into two subsectors $H = H_+ \oplus H_-$ with the conserved charge $\tau_3 = \pm 1$. The sub Hamiltonian is explicitly written as

$$H_{\tau=\pm}(\boldsymbol{k}) = v_\tau(s_+ k_y + s_- k_x) + M_z s_3, \quad v_\tau = v_1 + \tau v_2, \quad s_\pm = \frac{s_1 \pm s_2}{\sqrt{2}}. \tag{S.8}$$

The eigenvalue is given by $\pm E_\tau(\boldsymbol{k})$ with

$$E_\tau(\boldsymbol{k}) = \sqrt{v_\tau^2 k^2 + M_z^2}. \tag{S.9}$$

The corresponding eigenvector with the positive eigenvalue is given by

$$|\boldsymbol{k}\tau\rangle = \frac{1}{\sqrt{2}} \begin{pmatrix} e^{i(\pi/4-\phi_{\boldsymbol{k}})}\sqrt{1+\dfrac{M_z}{E_\tau(\boldsymbol{k})}} \\ \sqrt{1-\dfrac{M_z}{E_\tau(\boldsymbol{k})}} \end{pmatrix}, \tag{S.10}$$

where $\phi_{\boldsymbol{k}}$ denotes the angle of $\boldsymbol{k}$. By using PHS, one can obtain the eigenvector for the negative eigenvalue $-E_\tau(\boldsymbol{k})$ as $s_1 |-\boldsymbol{k}\tau\rangle^*$. The Hamiltonian is diagonalized to be

$$\hat{H} = \frac{1}{2}\sum_{\boldsymbol{k}\tau} \hat{\psi}^\dagger_{\boldsymbol{k}\tau} H_\tau(\boldsymbol{k}) \hat{\psi}_{\boldsymbol{k}\tau} = \sum_{\boldsymbol{k}\tau} E_\tau(\boldsymbol{k}) \gamma^\dagger_{\boldsymbol{k}\tau}\gamma_{\boldsymbol{k}\tau}, \tag{S.11}$$

with the Bogoliubov quasiparticle $\gamma_{\boldsymbol{k}\tau} = \langle \boldsymbol{k}\tau | \hat{\psi}_{\boldsymbol{k}\tau}$. The distribution is of Fermi statistics

$$\left\langle \gamma^\dagger_{\boldsymbol{k}\tau}\gamma_{\boldsymbol{k}'\tau'} \right\rangle = \delta_{\boldsymbol{k}\boldsymbol{k}'}\delta_{\tau\tau'} f(E_\tau(\boldsymbol{k})) = \delta_{\boldsymbol{k}\boldsymbol{k}'}\delta_{\tau\tau'} \frac{1}{e^{\beta E_\tau(\boldsymbol{k})}+1}. \tag{S.12}$$

### C. Spin

Spin operators are of $E$ irrep with PHS for $(\sigma^x, \sigma^y)$ and $A_2$ for $\sigma^z$ irrep with PHS, respectively. The spin from Majorana fermions is represented by

$$\frac{1}{2}\boldsymbol{\sigma} = \frac{1}{2}(\sigma^x, \sigma^y, \sigma^z) = \frac{1}{2}(\eta_5, \eta_6, -s_3\tau_0), \tag{S.13}$$

to satisfy $\{\sigma^i, \sigma^j\} = 2\delta^{ij}$ and $[\sigma^i, \sigma^j] = 2i\epsilon^{ijk}\sigma^k$.

Matrices $\eta_i$'s are defined by

$$\begin{aligned} \eta_1 &= \frac{1}{\sqrt{2}}(s_1\tau_0 + s_2\tau_0), \quad \eta_2 = \frac{-1}{\sqrt{2}}(s_1\tau_0 - s_2\tau_0), \quad \eta_3 = \frac{1}{\sqrt{2}}(s_1\tau_3 + s_2\tau_3), \quad \eta_4 = \frac{-1}{\sqrt{2}}(s_1\tau_3 - s_2\tau_3), \\ \eta_5 &= \frac{1}{\sqrt{2}}(s_1\tau_2 - s_2\tau_2), \quad \eta_6 = \frac{-1}{\sqrt{2}}(s_1\tau_2 + s_2\tau_2), \quad \eta_7 = \frac{1}{\sqrt{2}}(s_1\tau_1 - s_2\tau_1), \quad \eta_8 = \frac{-1}{\sqrt{2}}(s_1\tau_1 + s_2\tau_1). \end{aligned} \tag{S.14}$$

## II. SPIN CURRENT INDUCED BY DYNAMIC STRAIN

Impurity-averaged Green function for MFs is given by

$$G^{\mathrm{R/A}}_{\boldsymbol{k}}(\epsilon) = [\epsilon - H(\boldsymbol{k}) - \Sigma^{\mathrm{R/A}}(\epsilon)]^{-1}, \tag{S.15}$$

where we assume that the self energy is given by $\Sigma^{\mathrm{R/A}}(\epsilon) \equiv \mp i\gamma(\epsilon)$. Note that the chemical potential of MFs is equal to 0. The particle-hole symmetry is given by $C\Sigma^{\mathrm{R/A}}(\epsilon)C^{-1} = -\Sigma^{\mathrm{R/A}}(-\epsilon)$, $CG^{\mathrm{R/A}}_{\boldsymbol{k}}(\epsilon)C^{-1} = -G^{\mathrm{R/A}}_{-\boldsymbol{k}}(-\epsilon)$. Hence, $\Sigma^{\mathrm{R/A}}(0) = \mp i\gamma$ where we define $\gamma(0) = \gamma$ for leading order of $\epsilon$, and the real part of $\Sigma^{\mathrm{R/A}}(0)$ without particle-hole symmetry does not exist. Also, the time-reversal and chiral symmetries are given by $\Theta\Sigma^{\mathrm{R/A}}(\epsilon)\Theta^{-1} = \Sigma^{\mathrm{A/R}}(\epsilon)$, $\Theta G^{\mathrm{R/A}}_{\boldsymbol{k}}(\epsilon)\Theta^{-1} = G^{\mathrm{A/R}}_{-\boldsymbol{k}}(\epsilon)$ and $\Gamma\Sigma^{\mathrm{R/A}}(\epsilon)\Gamma^{-1} = -\Sigma^{\mathrm{A/R}}(-\epsilon)$, $\Gamma G^{\mathrm{R/A}}_{\boldsymbol{k}}(\epsilon)\Gamma^{-1} = -G^{\mathrm{A/R}}_{\boldsymbol{k}}(-\epsilon)$. We assume that this damping parameter takes nonzero value, and then we can use the condition $\omega \ll \tau^{-1} = 2\gamma$, where $\omega$ and $\tau$ denotes frequency of external field and relaxation time of the MFs.

### A. Spin current

We define spin current operators by

$$\hat{j}_i^\alpha(\boldsymbol{q}) = \frac{1}{2}\sum_{\boldsymbol{k}} \hat{\psi}^\dagger_{\boldsymbol{k}-\frac{\boldsymbol{q}}{2}} \frac{\{\sigma^\alpha/2, v_i\}}{2} \hat{\psi}_{\boldsymbol{k}+\frac{\boldsymbol{q}}{2}}, \quad v_i = \frac{\partial H(\boldsymbol{k})}{\partial k_i}, \tag{S.16}$$

from Eq. (S.13), and explicitly shown as

$$\hat{j}_x^x = -\hat{j}_y^y = \frac{1}{4}\sum_{\boldsymbol{k}} \hat{\psi}^\dagger_{\boldsymbol{k}-\boldsymbol{q}/2}(v_1 s_0 \tau_2)\hat{\psi}_{\boldsymbol{k}+\boldsymbol{q}/2}, \tag{S.17}$$

$$\hat{j}_x^y = \hat{j}_y^x = \frac{1}{4}\sum_{\boldsymbol{k}} \hat{\psi}^\dagger_{\boldsymbol{k}-\boldsymbol{q}/2}(-v_2 s_3 \tau_1)\hat{\psi}_{\boldsymbol{k}+\boldsymbol{q}/2}, \tag{S.18}$$

$$\hat{j}_x^z = \hat{j}_y^z = 0. \tag{S.19}$$

It is sufficient to focus on the following two components, which belong to $B_1$ and $B_2$ irreps.

$$\hat{B}^{(1)}(\boldsymbol{q}) \equiv \hat{j}_y^x(\boldsymbol{q}) + \hat{j}_x^y(\boldsymbol{q}) = \frac{1}{2}\sum_{\boldsymbol{k}} \hat{\psi}^\dagger_{\boldsymbol{k}-\frac{\boldsymbol{q}}{2}}[-v_2 s_3 \tau_1]\hat{\psi}_{\boldsymbol{k}+\frac{\boldsymbol{q}}{2}} \equiv \frac{1}{2}\sum_{\boldsymbol{k}} \hat{\psi}^\dagger_{\boldsymbol{k}-\frac{\boldsymbol{q}}{2}}[b^{(1)}]\hat{\psi}_{\boldsymbol{k}+\frac{\boldsymbol{q}}{2}}, \tag{S.20}$$

$$\hat{B}^{(2)}(\boldsymbol{q}) \equiv \hat{j}_x^x(\boldsymbol{q}) - \hat{j}_y^y(\boldsymbol{q}) = \frac{1}{2}\sum_{\boldsymbol{k}} \hat{\psi}^\dagger_{\boldsymbol{k}-\frac{\boldsymbol{q}}{2}}[v_1 s_0 \tau_2]\hat{\psi}_{\boldsymbol{k}+\frac{\boldsymbol{q}}{2}} \equiv \frac{1}{2}\sum_{\boldsymbol{k}} \hat{\psi}^\dagger_{\boldsymbol{k}-\frac{\boldsymbol{q}}{2}}[b^{(2)}]\hat{\psi}_{\boldsymbol{k}+\frac{\boldsymbol{q}}{2}}. \tag{S.21}$$

### B. dynamic strain

The dynamic strain is expressed by the unsymmetrized tensor $u_{ij}(\boldsymbol{r},t) = \partial_i u_j(\boldsymbol{r},t)$, which is coupled to the physical observables when they belong to the same irrep. From Table I, there are only two operators of $B_1$ and $B_2$ irreps with time-reversal and particle-hole symmetries. They couple with applied dynamic strains as

$$\hat{H}_{\mathrm{ext}}(t) = -\int d^2\boldsymbol{r} \left\{ \hat{O}^{(1)}(\boldsymbol{r})[u_{xx}(\boldsymbol{r},t) - u_{yy}(\boldsymbol{r},t)] + \hat{O}^{(2)}(\boldsymbol{r})[u_{xy}(\boldsymbol{r},t) + u_{yx}(\boldsymbol{r},t)] \right\}, \tag{S.22}$$

$$\hat{O}^{(1)}(\boldsymbol{r}) \equiv \frac{1}{2}\hat{\psi}^\dagger(\boldsymbol{r})(\rho_1 s_3 \tau_1)\hat{\psi}(\boldsymbol{r}),\ \hat{O}^{(2)}(\boldsymbol{r}) \equiv \frac{1}{2}\hat{\psi}^\dagger(\boldsymbol{r})(\rho_2 s_0 \tau_2)\hat{\psi}(\boldsymbol{r}), \tag{S.23}$$

where we define $\psi(\boldsymbol{r}) = \sum_{\boldsymbol{k}} e^{i\boldsymbol{k}\cdot\boldsymbol{r}}\psi_{\boldsymbol{k}}$ and $\hat{O}^{(i)}(\boldsymbol{r}) \equiv \frac{1}{2}\hat{\psi}^\dagger(\boldsymbol{r})(o^{(i)})\hat{\psi}(\boldsymbol{r})$. The other modes of strains appear in the higher orders of gradient, which would be irrelevant in the low-energy regime.

The response functions of spin current are defined by

$$K_{ij}(\boldsymbol{q},\omega) \equiv i\int_0^\infty dt e^{i(\omega+i\delta)t}\, \langle[\hat{B}^{(i)}(\boldsymbol{q},t), \hat{O}^{(j)}(-\boldsymbol{q},0)]\rangle, \quad \hat{O}^{(j)}(\boldsymbol{q}) = \frac{1}{2}\sum_{\boldsymbol{k}} \hat{\psi}^\dagger_{\boldsymbol{k}-\frac{\boldsymbol{q}}{2}} o^{(j)} \hat{\psi}_{\boldsymbol{k}+\frac{\boldsymbol{q}}{2}}, \tag{S.24}$$

where $\hat{A}(t) = e^{iHt}\hat{A}e^{-iHt}$ and $\delta \to +0$. Also, $\langle\cdots\rangle = \mathrm{tr}[e^{-H/T}\cdots]/\mathrm{tr}[e^{-H/T}]$. Then, the spin currents are given by

$$\langle \hat{j}_y^x(\boldsymbol{q},\omega) + \hat{j}_x^y(\boldsymbol{q},\omega)\rangle = K_{11}(\boldsymbol{q},\omega)[u_{xx}(\boldsymbol{q},\omega) - u_{yy}(\boldsymbol{q},\omega)] + K_{12}(\boldsymbol{q},\omega)[u_{xy}(\boldsymbol{q},\omega) + u_{yx}(\boldsymbol{q},\omega)], \tag{S.25}$$

$$\langle \hat{j}_x^x(\boldsymbol{q},\omega) - \hat{j}_y^y(\boldsymbol{q},\omega)\rangle = K_{21}(\boldsymbol{q},\omega)[u_{xx}(\boldsymbol{q},\omega) - u_{yy}(\boldsymbol{q},\omega)] + K_{22}(\boldsymbol{q},\omega)[u_{xy}(\boldsymbol{q},\omega) + u_{yx}(\boldsymbol{q},\omega)]. \tag{S.26}$$

The Matsubara representation response functions are given by

$$K_{ij}(\boldsymbol{q}, i\omega_l) = \int_0^{1/T} d\tau e^{i\omega_l\tau}\langle T_\tau(\hat{B}^{(i)}(\boldsymbol{q},\tau))\hat{O}^{(j)}(-\boldsymbol{q},0)\rangle, \tag{S.27}$$

where $\omega_l = 2l\pi T$ is the bosonic Matsubara frequency. By using the Wick's theorem, the response functions are

reduced as follows.

$$
\begin{aligned}
K_{ij}(\boldsymbol{q}, i\omega_l) &= \int_0^{1/T} d\tau e^{i\omega_l \tau} \langle T_\tau (\hat{B}^{(i)}(\boldsymbol{q},\tau)) \hat{O}^{(j)}(-\boldsymbol{q},0)\rangle \\
&= \frac{1}{4}\sum_{\boldsymbol{k},\boldsymbol{k}'} \int_0^{1/T} d\tau e^{i\omega_l\tau} \langle T_\tau \hat{\psi}^\dagger_{\boldsymbol{k}-\frac{\boldsymbol{q}}{2},\alpha}(\tau) b^{(i)}_{\alpha\beta} \hat{\psi}_{\boldsymbol{k}+\frac{\boldsymbol{q}}{2},\beta}(\tau) \hat{\psi}^\dagger_{\boldsymbol{k}'+\frac{\boldsymbol{q}}{2},\gamma}(0) o^{(j)}_{\gamma\eta} \hat{\psi}_{\boldsymbol{k}'-\frac{\boldsymbol{q}}{2},\eta}(0)\rangle \\
&= \frac{1}{4}\sum_{\boldsymbol{k},\boldsymbol{k}'} \int_0^{1/T} d\tau e^{i\omega_l\tau} \Bigg[ - b^{(i)}_{\alpha\beta} o^{(j)}_{\gamma\eta} \langle T_\tau \hat{\psi}^\dagger_{\boldsymbol{k}-\frac{\boldsymbol{q}}{2},\alpha}(\tau) \hat{\psi}^\dagger_{\boldsymbol{k}'+\frac{\boldsymbol{q}}{2},\gamma}(0)\rangle \langle T_\tau \hat{\psi}_{\boldsymbol{k}+\frac{\boldsymbol{q}}{2},\beta}(\tau) \hat{\psi}_{\boldsymbol{k}'-\frac{\boldsymbol{q}}{2},\eta}(0)\rangle \\
&\qquad\qquad + b^{(i)}_{\alpha\beta} o^{(j)}_{\gamma\eta} \langle T_\tau \hat{\psi}^\dagger_{\boldsymbol{k}-\frac{\boldsymbol{q}}{2},\alpha}(\tau) \hat{\psi}_{\boldsymbol{k}'-\frac{\boldsymbol{q}}{2},\eta}(0)\rangle \langle T_\tau \hat{\psi}_{\boldsymbol{k}+\frac{\boldsymbol{q}}{2},\beta}(\tau) \hat{\psi}^\dagger_{\boldsymbol{k}'+\frac{\boldsymbol{q}}{2},\gamma}(0)\rangle \Bigg]. \qquad \text{(S.28)}
\end{aligned}
$$

The first term reduces to

$$
\begin{aligned}
&\sum_{\boldsymbol{k},\boldsymbol{k}'} b^{(i)}_{\alpha\beta} o^{(j)}_{\gamma\eta} \left\langle T_\tau \hat{\psi}^\dagger_{\boldsymbol{k}-\boldsymbol{q}/2,\alpha}(\tau) \hat{\psi}^\dagger_{\boldsymbol{k}'+\boldsymbol{q}/2,\gamma}(0)\right\rangle \left\langle T_\tau \hat{\psi}_{\boldsymbol{k}+\boldsymbol{q}/2,\beta}(\tau) \hat{\psi}_{\boldsymbol{k}'-\boldsymbol{q}/2,\eta}(0)\right\rangle \\
&= \sum_{\boldsymbol{k},\boldsymbol{k}'} (s_1\tau_0)_{\alpha'\alpha} b^{(i)}_{\alpha\beta} (s_1\tau_0)_{\beta\beta'} o^{(j)}_{\gamma\eta} \left\langle T_\tau \hat{\psi}_{-\boldsymbol{k}+\boldsymbol{q}/2,\alpha'}(\tau) \hat{\psi}^\dagger_{\boldsymbol{k}'+\boldsymbol{q}/2,\gamma}(0)\right\rangle \left\langle T_\tau \hat{\psi}^\dagger_{-\boldsymbol{k}-\boldsymbol{q}/2,\beta'}(\tau) \hat{\psi}_{\boldsymbol{k}'-\boldsymbol{q}/2,\eta}(0)\right\rangle \\
&= \sum_{\boldsymbol{k}} b^{(i)}_{\beta\alpha} o^{(j)}_{\gamma\eta} [G_{-\boldsymbol{k}+\boldsymbol{q}/2}(\tau)]_{\alpha,\gamma} [G_{-\boldsymbol{k}-\boldsymbol{q}/2}(-\tau)]_{\eta,\beta} \\
&= \sum_{\boldsymbol{k}} \mathrm{tr}\Big[b^{(i)} G_{\boldsymbol{k}+\boldsymbol{q}/2}(\tau) o^{(j)} G_{\boldsymbol{k}-\boldsymbol{q}/2}(-\tau)\Big],
\end{aligned}
$$

where we define $[G_{\boldsymbol{k}}(\tau)]_{\alpha\beta} = -\langle T_\tau \hat{\psi}_{\boldsymbol{k},\alpha}(\tau)\hat{\psi}^\dagger_{\boldsymbol{k},\beta}(0)\rangle$ and use PHS $\hat{\psi}_{\boldsymbol{k}\alpha} = (s_1\tau_0)_{\alpha\alpha'}\hat{\psi}^\dagger_{-\boldsymbol{k}\alpha'}$, $\hat{\psi}^\dagger_{\boldsymbol{k}\alpha} = (s_1\tau_0)_{\alpha\alpha'}\hat{\psi}_{-\boldsymbol{k}\alpha'}$, and $(s_1\tau_0)b^{(i)}(s_1\tau_0) = -(b^{(i)})^* = -(b^{(i)})^{\mathrm{T}}$. The second term of Eq. (S.28) reduces to the same expression above. As a result,

$$
\begin{aligned}
K_{ij}(\boldsymbol{q}, i\omega_l) &= -\frac{1}{2}\sum_{\boldsymbol{k}} \int_0^{1/T} d\tau e^{i\omega_l\tau}\, \mathrm{tr}\Big[b^{(i)} G_{\boldsymbol{k}+\frac{\boldsymbol{q}}{2}}(\tau) o^{(j)} G_{\boldsymbol{k}-\frac{\boldsymbol{q}}{2}}(-\tau)\Big] \qquad \text{(S.29)} \\
&= -\frac{1}{2}\sum_{\boldsymbol{k}} T \sum_n \mathrm{tr}\Big[b^{(i)} G_{\boldsymbol{k}+\frac{\boldsymbol{q}}{2}}(i\epsilon_n + i\omega_l) o^{(j)} G_{\boldsymbol{k}-\frac{\boldsymbol{q}}{2}}(i\epsilon_n)\Big]. \qquad \text{(S.30)}
\end{aligned}
$$

where $G(\tau) = T\sum_n e^{-i\epsilon_n\tau}G(i\epsilon_n)$ for $\epsilon_n = 2(n+1)\pi T$.

We can expand the response function in terms of $\omega$ for $\omega \ll \tau^{-1} = 2\gamma$: $K_{ij}(\boldsymbol{q},\omega) = K^{(0)}_{ij}(\boldsymbol{q}) + \omega K^{(1)}_{ij}(\boldsymbol{q}) + \cdots$. The zeroth order $K^{(0)}$ is just the equilibrium contribution, discarded in this study. The first order $K^{(1)}$ is the leading term of the nonequilibrium contribution, which is decomposed into Fermi-sea $K^{\mathrm{sea}}_{ij}$ and Fermi-surface $K^{\mathrm{sf},CC'}_{ij}$ terms [8]

$$
K^{(1)}_{ij}(\boldsymbol{q}) \equiv K^{\mathrm{sf,RA}}_{ij}(\boldsymbol{q}) - \frac{1}{2}\Big(K^{\mathrm{sf,RR}}_{ij}(\boldsymbol{q}) + K^{\mathrm{sf,AA}}_{ij}(\boldsymbol{q})\Big) + K^{\mathrm{sea}}_{ij}(\boldsymbol{q}), \qquad \text{(S.31)}
$$

defined by

$$
\begin{aligned}
K^{\mathrm{sea}}_{ij}(\boldsymbol{q}) &= \frac{i}{8\pi}\sum_{\boldsymbol{k}} \int_{-\infty}^0 d\epsilon \lim_{\epsilon'\to\epsilon} (\partial_\epsilon - \partial_{\epsilon'}) \times \Big\{\mathrm{tr}\big[\,\big(b^{(i)}\big) G^{\mathrm{R}}_{\boldsymbol{k}}(\epsilon') \big(o^{(j)}\big) G^{\mathrm{R}}_{\boldsymbol{k}}(\epsilon)\big] - \langle \mathrm{R} \leftrightarrow \mathrm{A}\rangle\Big\}, \qquad \text{(S.32)} \\
K^{\mathrm{sf,RA}}_{ij}(\boldsymbol{q}) &= \frac{i}{4\pi}\sum_{\boldsymbol{k}} \mathrm{tr}\Big[\,\big(b^{(i)}\big) G^{\mathrm{R}}_{\boldsymbol{k}+\frac{\boldsymbol{q}}{2}}(0) \big(o^{(j)}\big) G^{\mathrm{A}}_{\boldsymbol{k}-\frac{\boldsymbol{q}}{2}}(0)\Big], \qquad \text{(S.33)} \\
K^{\mathrm{sf,CC}}_{ij}(\boldsymbol{q}) &= \frac{i}{4\pi}\sum_{\boldsymbol{k}} \mathrm{tr}\Big[\,\big(b^{(i)}\big) G^{\mathrm{C}}_{\boldsymbol{k}+\frac{\boldsymbol{q}}{2}}(0) \big(o^{(j)}\big) G^{\mathrm{C}}_{\boldsymbol{k}-\frac{\boldsymbol{q}}{2}}(0)\Big], \qquad \text{(S.34)}
\end{aligned}
$$

where C = R or A. Then, the spin current is given by

$$
\langle \hat{j}^x_y(\boldsymbol{q},\omega) + \hat{j}^y_x(\boldsymbol{q},\omega)\rangle = (K^{(0)}_{11} + \omega K^{(1)}_{11} + \cdots)[u_{xx}(\boldsymbol{q},\omega) - u_{yy}(\boldsymbol{q},\omega)] + (K^{(0)}_{12} + \omega K^{(1)}_{12} + \cdots)[u_{xy}(\boldsymbol{q},\omega) + u_{yx}(\boldsymbol{q},\omega)], \qquad \text{(S.35)}
$$

$$
\langle \hat{j}^x_x(\boldsymbol{q},\omega) - \hat{j}^y_y(\boldsymbol{q},\omega)\rangle = (K^{(0)}_{21} + \omega K^{(1)}_{21} + \cdots)[u_{xx}(\boldsymbol{q},\omega) - u_{yy}(\boldsymbol{q},\omega)] + (K^{(0)}_{22} + \omega K^{(1)}_{22} + \cdots)[u_{xy}(\boldsymbol{q},\omega) + u_{yx}(\boldsymbol{q},\omega)]. \qquad \text{(S.36)}
$$

### C. Calculation of $K_{ij}^{(1)}$ in the case of $M_z = 0$

Here we assume that the wavenumber of the strains $q$ are small with respect to the mean free path $l$ of the MFs. The condition is represented by $q \ll l^{-1}$ and we neglect $\boldsymbol{q}$ dependence. For $b^{(i)}$ and $o^{(j)}$, if $i = j$, they are same matrix representaion and then

$$K_{ii}^{\rm sea} = \frac{i}{8\pi}\sum_{\boldsymbol{k}}\int_{-\infty}^{0} d\epsilon \lim_{\epsilon'\to\epsilon}(\partial_\epsilon - \partial_{\epsilon'}) \times \Big\{{\rm tr}\big[(b^{(i)})G_{\boldsymbol{k}}^{\rm R}(\epsilon')(o^{(i)})G_{\boldsymbol{k}}^{\rm R}(\epsilon)\big] - \langle {\rm R} \leftrightarrow {\rm A}\rangle\Big\} = 0. \tag{S.37}$$

And, if $i \neq j$, $b^{(i)}$ and $o^{(j)}$ have the different sign character for mirror symmetry $\sigma(xz)$ each other,

$$\begin{aligned}
K_{ij}^{\rm sea} &= \frac{i}{8\pi}\sum_{\boldsymbol{k}}\int_{-\infty}^{0} d\epsilon \lim_{\epsilon'\to\epsilon}(\partial_\epsilon - \partial_{\epsilon'}) \times \Big\{{\rm tr}\big[(b^{(i)})G_{\boldsymbol{k}}^{\rm R}(\epsilon')(o^{(j)})G_{\boldsymbol{k}}^{\rm R}(\epsilon)\big] - \langle {\rm R} \leftrightarrow {\rm A}\rangle\Big\} \\
&= \frac{i}{8\pi}\sum_{\boldsymbol{k}}\int_{-\infty}^{0} d\epsilon \lim_{\epsilon'\to\epsilon}(\partial_\epsilon - \partial_{\epsilon'}) \times \Big\{{\rm tr}\big[-(b^{(i)})G_{k_x,-k_y}^{\rm R}(\epsilon')(o^{(j)})G_{k_x,-k_y}^{\rm R}(\epsilon)\big] + \langle {\rm R} \leftrightarrow {\rm A}\rangle\Big\} \\
&= \frac{i}{8\pi}\sum_{\boldsymbol{k}}\int_{-\infty}^{0} d\epsilon \lim_{\epsilon'\to\epsilon}(\partial_\epsilon - \partial_{\epsilon'}) \times \Big\{{\rm tr}\big[-(b^{(i)})G_{\boldsymbol{k}}^{\rm R}(\epsilon')(o^{(j)})G_{\boldsymbol{k}}^{\rm R}(\epsilon)\big] + \langle {\rm R} \leftrightarrow {\rm A}\rangle\Big\} \\
&= -K_{ij}^{\rm sea},
\end{aligned} \tag{S.38}$$

Therefore $K_{ij}^{\rm sea} = 0$ and then $K_{12} = K_{21} = 0$. Also, we calculate

$$K_{ij}^{\rm sf,RA} = \frac{i}{4\pi}\sum_{\boldsymbol{k}}{\rm tr}\Big[(b^{(i)})G_{\boldsymbol{k}}^{\rm R}(0)(o^{(j)})G_{\boldsymbol{k}}^{\rm A}(0)\Big], \tag{S.39}$$

$$K_{ij}^{\rm sf,CC} = \frac{i}{4\pi}\sum_{\boldsymbol{k}}{\rm tr}\Big[(b^{(i)})G_{\boldsymbol{k}}^{\rm C}(0)(o^{(j)})G_{\boldsymbol{k}}^{\rm C}(0)\Big]. \tag{S.40}$$

Then, $K_{11}^{\rm sf,RA} - (K_{11}^{\rm sf,RR} + K_{11}^{\rm sf,AA})/2$ is given by

$$\frac{i}{4\pi}\left(\frac{1}{2\pi}\right)^2(2\pi)\frac{\rho_1}{v_1}\ln\left[\frac{(v_1-v_2)^2}{(v_1+v_2)^2}\right], \tag{S.41}$$

where this result includes contributions of the $K_{11}^{\rm sf,RR}$ and $K_{11}^{\rm sf,AA}$. On the other hand, $K_{22}^{\rm sf,RA} - (K_{22}^{\rm sf,RR} + K_{22}^{\rm sf,AA})/2$ is given by

$$\frac{i}{4\pi}\left(\frac{1}{2\pi}\right)^2(2\pi)\frac{-\rho_2}{v_2}\ln\left[\frac{(v_1-v_2)^2}{(v_1+v_2)^2}\right]. \tag{S.42}$$

One finds the relation $K_{22}^{(1)} = \frac{v_1\rho_2}{-v_2\rho_1}K_{11}^{(1)}$ from Eqs. (S.41) and (S.42), which is a consequence from the mirror and chiral symmetries, as shown below.

$$\begin{aligned}
K_{22}^{\rm sf,RA} &= \frac{i}{4\pi}\sum_{\boldsymbol{k}}{\rm tr}\Big[(v_1 s_0\tau_2)G_{\boldsymbol{k}}^{\rm R}(0)(\rho_2 s_0\tau_2)G_{\boldsymbol{k}}^{\rm A}(0)\Big] \\
&= \frac{i}{4\pi}\frac{1}{2}\left(\sum_{\boldsymbol{k}}{\rm tr}\Big[(v_1(is_3\tau_1\Gamma))G_{\boldsymbol{k}}^{\rm R}(0)(\rho_2(-i\Gamma s_3\tau_1))G_{\boldsymbol{k}}^{\rm A}(0)\Big] + \sum_{\boldsymbol{k}}{\rm tr}\Big[(v_1(-i\Gamma s_3\tau_1))G_{\boldsymbol{k}}^{\rm R}(0)(\rho_2(is_3\tau_1\Gamma))G_{\boldsymbol{k}}^{\rm A}(0)\Big]\right) \\
&= \frac{i}{4\pi}\frac{1}{2}\left(\sum_{\boldsymbol{k}}{\rm tr}\Big[(v_1 s_3\tau_1)\Gamma G_{\boldsymbol{k}}^{\rm R}(0)\Gamma^{-1}(\rho_2 s_3\tau_1)G_{\boldsymbol{k}}^{\rm A}(0)\Big] + \sum_{\boldsymbol{k}}{\rm tr}\Big[(v_1 s_3\tau_1)G_{\boldsymbol{k}}^{\rm R}(0)(\rho_2 s_3\tau_1)\Gamma G_{\boldsymbol{k}}^{\rm A}(0)\Gamma^{-1}\Big]\right) \\
&= \frac{i}{4\pi}\frac{1}{2}\left(\sum_{\boldsymbol{k}}{\rm tr}\Big[(v_1 s_3\tau_1)(-G_{\boldsymbol{k}}^{\rm A}(0))(\rho_2 s_3\tau_1)G_{\boldsymbol{k}}^{\rm A}(0)\Big] + \sum_{\boldsymbol{k}}{\rm tr}\Big[(v_1 s_3\tau_1)G_{\boldsymbol{k}}^{\rm R}(0)(\rho_2 s_3\tau_1)(-G_{\boldsymbol{k}}^{\rm R}(0))\Big]\right) \\
&= \frac{v_1\rho_2}{-v_2\rho_1}\big[-(K_{11}^{\rm sf,RR} + K_{11}^{\rm sf,AA})/2\big],
\end{aligned} \tag{S.43}$$

with the help of chiral symmetry for the Green's function $\Gamma G_{\boldsymbol{k}}^{\mathrm{R/A}}(0)\Gamma^{-1} = -G_{\boldsymbol{k}}^{\mathrm{A/R}}(0)$, $\Gamma = s_3\tau_3$ defined by Eq. (S.3). We also use $s_0\tau_2 = -i\Gamma s_3\tau_1 = is_3\tau_1\Gamma$. In a similar way, we get

$$K_{11}^{\mathrm{sf,RA}} = \frac{1}{2}\frac{v_2\rho_1}{-v_1\rho_2}\Big[-(K_{22}^{\mathrm{sf,RR}} + K_{22}^{\mathrm{sf,AA}})\Big]. \tag{S.44}$$

Therefore, we find the relation for the response function $K_{ii}^{(1)}$ [Eq. (S.31)] with $K_{ii}^{\mathrm{sea}} = 0$

$$\begin{aligned} K_{22}^{(1)} &= K_{22}^{\mathrm{sf,RA}} - (K_{22}^{\mathrm{sf,RR}} + K_{22}^{\mathrm{sf,AA}})/2 \\ &= \frac{v_1\rho_2}{-v_2\rho_1}\big[-(K_{11}^{\mathrm{sf,RR}} + K_{11}^{\mathrm{sf,AA}})/2\big] + \frac{v_1\rho_2}{-v_2\rho_1}K_{11}^{\mathrm{sf,RA}} = \frac{v_1\rho_2}{-v_2\rho_1}K_{11}^{(1)}. \end{aligned} \tag{S.45}$$

### D. Calculation of $K_{ij}^{(1)}$ in the case of $M_z \neq 0$

We calculate

$$K_{ij}^{\mathrm{sea}} = \frac{i}{8\pi}\sum_{\boldsymbol{k}}\int_{-\infty}^{0} d\epsilon \lim_{\epsilon'\to\epsilon}(\partial_\epsilon - \partial_{\epsilon'}) \times \Big\{\mathrm{tr}\big[(b^{(i)})G_{\boldsymbol{k}}^{\mathrm{R}}(\epsilon')(o^{(j)})G_{\boldsymbol{k}}^{\mathrm{R}}(\epsilon)\big] - \langle \mathrm{R}\leftrightarrow\mathrm{A}\rangle\Big\} = 0 \tag{S.46}$$

since the same reason as Eqs. (S.37) and (S.38) for $i = j$. The magnetization $M_z$ breaks mirror symmetry $\sigma(xz)$, however, the system still has magnetic mirror symmetry $\Theta\sigma(xz)$. Therefore, one can find

$$\begin{aligned} K_{ij}^{\mathrm{sea}} &= \frac{i}{8\pi}\sum_{\boldsymbol{k}}\int_{-\infty}^{0} d\epsilon \lim_{\epsilon'\to\epsilon}(\partial_\epsilon - \partial_{\epsilon'}) \times \Big\{\mathrm{tr}\big[(b^{(i)})G_{\boldsymbol{k}}^{\mathrm{R}}(\epsilon')(o^{(j)})G_{\boldsymbol{k}}^{\mathrm{R}}(\epsilon)\big] - \langle \mathrm{R}\leftrightarrow\mathrm{A}\rangle\Big\} \\ &= \frac{-i}{8\pi}\sum_{\boldsymbol{k}}\int_{-\infty}^{0} d\epsilon \lim_{\epsilon'\to\epsilon}(\partial_\epsilon - \partial_{\epsilon'}) \times \Big\{\mathrm{tr}\big[-(b^{(i)})G_{-k_x,k_y}^{\mathrm{A}}(\epsilon')(o^{(j)})G_{-k_x,k_y}^{\mathrm{A}}(\epsilon)\big] + \langle \mathrm{A}\leftrightarrow\mathrm{R}\rangle\Big\} \\ &= \frac{i}{8\pi}\sum_{\boldsymbol{k}}\int_{-\infty}^{0} d\epsilon \lim_{\epsilon'\to\epsilon}(\partial_\epsilon - \partial_{\epsilon'}) \times \Big\{\mathrm{tr}\big[-(b^{(i)})G_{\boldsymbol{k}}^{\mathrm{R}}(\epsilon')(o^{(j)})G_{\boldsymbol{k}}^{\mathrm{R}}(\epsilon)\big] + \langle \mathrm{R}\leftrightarrow\mathrm{A}\rangle\Big\} \\ &= -K_{ij}^{\mathrm{sea}}, \end{aligned} \tag{S.47}$$

where we use $\Theta b^{(i)}\Theta^{-1} = b^{(i)}$, $\Theta o^{(j)}\Theta^{-1} = o^{(j)}$. As a result, $K_{ij}^{\mathrm{sea}} = 0$ and then $K_{12}^{\mathrm{sea}} = K_{21}^{\mathrm{sea}} = 0$ for $M_z \neq 0$. Also, we calculate

$$K_{ij}^{\mathrm{sf,RA}} = \frac{i}{4\pi}\sum_{\boldsymbol{k}}\mathrm{tr}\Big[(b^{(i)})G_{\boldsymbol{k}}^{\mathrm{R}}(0)(o^{(j)})G_{\boldsymbol{k}}^{\mathrm{A}}(0)\Big], \tag{S.48}$$

$$K_{ij}^{\mathrm{sf,CC}} = \frac{i}{4\pi}\sum_{\boldsymbol{k}}\mathrm{tr}\Big[(b^{(i)})G_{\boldsymbol{k}}^{\mathrm{C}}(0)(o^{(j)})G_{\boldsymbol{k}}^{\mathrm{C}}(0)\Big], \tag{S.49}$$

where we neglect $\boldsymbol{q}$ dependence. Then, $K_{11}^{\mathrm{sf,RA}} - (K_{11}^{\mathrm{sf,RR}} + K_{11}^{\mathrm{sf,AA}})/2$ is given by

$$\frac{i}{4\pi}\left(\frac{1}{2\pi}\right)^2(2\pi)\frac{\gamma^2}{M_z^2+\gamma^2}\frac{\rho_1}{v_1}\ln\left[\frac{(v_1-v_2)^2}{(v_1+v_2)^2}\right], \tag{S.50}$$

where this result includes contributions of the $K_{11}^{\mathrm{sf,RR}}$ and $K_{11}^{\mathrm{sf,AA}}$. On the other hand, $K_{22}^{\mathrm{sf,RA}} - (K_{22}^{\mathrm{sf,RR}} + K_{22}^{\mathrm{sf,AA}})/2$ is given by

$$\frac{i}{4\pi}\left(\frac{1}{2\pi}\right)^2(2\pi)\frac{\gamma^2}{M_z^2+\gamma^2}\frac{-\rho_2}{v_2}\ln\left[\frac{(v_1-v_2)^2}{(v_1+v_2)^2}\right]. \tag{S.51}$$

Here, $K_{12}(\omega)$ ($K_{21}(\omega)$) can take finite value in the case of $M_z \neq 0$ since the applied magnetization lowers the symmetry from $C_{4v}$ to $C_4$, and $j_y^x + j_x^y$ and $u_{xy} + u_{yx}$ share the same irreducible representation of $C_4$. The calculations are shown as followings.

### E. Calculation of $K_{11}(\omega)$ and $K_{12}(\omega)$ from Lehmann representation in the case of $M_z \neq 0$

We calculate $K_{11}(\omega)$ and $K_{12}(\omega)$ from the Lehmann representation:

$$K_{11}(\omega) = \frac{1}{4} \sum_{n\in\text{occ},m\in\text{unocc}} \left\{ \frac{\langle n| - v_2 s_3\tau_1|m\rangle\langle m|\rho_1 s_3\tau_1|n\rangle}{E_n - E_m + \omega + i\delta} + \left[ \frac{\langle n| - v_2 s_3\tau_1|m\rangle\langle m|\rho_1 s_3\tau_1|n\rangle}{E_n - E_m - \omega + i\delta} \right]^* \right\}, \tag{S.52}$$

$$K_{12}(\omega) = \frac{1}{4} \sum_{n\in\text{occ},m\in\text{unocc}} \left\{ \frac{\langle n| - v_2 s_3\tau_1|m\rangle\langle m|\rho_2 s_0\tau_2|n\rangle}{E_n - E_m + \omega + i\delta} + \left[ \frac{\langle n| - v_2 s_3\tau_1|m\rangle\langle m|\rho_2 s_0\tau_2|n\rangle}{E_n - E_m - \omega + i\delta} \right]^* \right\}, \tag{S.53}$$

where the chemical potential of MFs is equal to 0 owing to particle-hole symmetry. Note that Eq. (S.6) can be rewrite $H = H_+ \oplus H_-$, and $H_{\tau=\pm}$ where $\tau$ is the eigenvalue of $\tau_3$ is given by

$$H_\tau = \boldsymbol{d}_\tau(\boldsymbol{k}) \cdot \boldsymbol{s} = \begin{pmatrix} M_z & \frac{1+i}{\sqrt{2}}(k_x - ik_y)(v_1 + \tau v_2) \\ \text{h.c.} & -M_z \end{pmatrix}, \tag{S.54}$$

$$d_{\tau,x} = \frac{k_x}{\sqrt{2}}(v_1 + \tau v_2) + \frac{k_y}{\sqrt{2}}(v_1 + \tau v_2), \; d_{\tau,y} = -\frac{k_x}{\sqrt{2}}(v_1 + \tau v_2) + \frac{k_y}{\sqrt{2}}(v_1 + \tau v_2), \; d_{\tau,z} = M_z, \tag{S.55}$$

where the eigenvectors of $H_\tau$ corresponding to the four eigenvalues of Eq. (S.6), $E_{\tau,\pm} = \pm\sqrt{M_z^2 + k^2(v_1 + \tau v_2)^2}$, are given by

$$|\tau+\rangle = \begin{pmatrix} \cos(\theta_\tau/2) \\ e^{i\phi_\tau}\sin(\theta_\tau/2) \end{pmatrix}, \quad |\tau-\rangle = \begin{pmatrix} \sin(\theta_\tau/2) \\ -e^{i\phi_\tau}\cos(\theta_\tau/2) \end{pmatrix}, \tag{S.56}$$

$$\cos(\theta_\tau) = \frac{d_{\tau,z}}{E_{\tau,+}}, \; \sin(\theta_\tau)\cos(\phi_\tau) = \frac{d_{\tau,x}}{E_{\tau,+}}, \; \sin(\theta_\tau)\sin(\phi_\tau) = \frac{d_{\tau,y}}{E_{\tau,+}}. \tag{S.57}$$

#### 1. $K_{11}(\omega)$

In the next, we calculate the firtst term of Eq. (S.52) and omit $\frac{1}{4}$ and $+i\delta$:

$$\begin{aligned} &\sum_{n\in\text{occ},m\in\text{unocc}} \frac{\langle n| - v_2 s_3\tau_1|m\rangle\langle m|\rho_1 s_3\tau_1|n\rangle}{E_n - E_m + \omega} \\ &= -v_2\rho_1 \left[ \frac{(\tau_1)_{11}\langle +-|s_3|++\rangle\langle ++|s_3|+-\rangle(\tau_1)_{11}}{E_{+,-} - E_{+,+} + \omega} + \frac{(\tau_1)_{12}\langle +-|s_3|-+\rangle\langle -+|s_3|+-\rangle(\tau_1)_{21}}{E_{+,-} - E_{-,+} + \omega} \right. \\ &\qquad \left. + \frac{(\tau_1)_{21}\langle --|s_3|++\rangle\langle ++|s_3|--\rangle(\tau_1)_{12}}{E_{-,-} - E_{+,+} + \omega} + \frac{(\tau_1)_{22}\langle --|s_3|-+\rangle\langle -+|s_3|--\rangle(\tau_1)_{22}}{E_{-,-} - E_{-,+} + \omega} \right] \\ &= -v_2\rho_1 \left[ \frac{(\tau_1)_{12}\langle +-|s_3|-+\rangle\langle -+|s_3|+-\rangle(\tau_1)_{21}}{E_{+,-} - E_{-,+} + \omega} + \frac{(\tau_1)_{21}\langle --|s_3|++\rangle\langle ++|s_3|--\rangle(\tau_1)_{12}}{E_{-,-} - E_{+,+} + \omega} \right] \\ &= -v_2\rho_1 \left[ \frac{\langle +-|s_3|-+\rangle\langle -+|s_3|+-\rangle}{E_{+,-} - E_{-,+} + \omega} + \frac{\langle --|s_3|++\rangle\langle ++|s_3|--\rangle}{E_{+,-} - E_{-,+} + \omega} \right], \end{aligned} \tag{S.58}$$

where we use $E_{-,-} = -E_{-,+}, E_{+,+} = -E_{+,-}$. By using Eq. (S.55)–(S.57), we get

$$\begin{aligned} &\sum_{n\in\text{occ},m\in\text{unocc}} \frac{\langle n| - v_2 s_3\tau_1|m\rangle\langle m|\rho_1 s_3\tau_1|n\rangle}{E_n - E_m + \omega} \\ &= -\frac{v_2\rho_1}{E_{+,-} - E_{-,+} + \omega} \left[ 2\sin^2(\theta_+/2)\cos^2(\theta_-/2) + 2\sin^2(\theta_-/2)\cos^2(\theta_+/2) + \cos(\phi_+ - \phi_-)\sin(\theta_+)\sin(\theta_-) \right]. \end{aligned} \tag{S.59}$$

Then, the response function is given by

$$K_{11}(\omega) = -\frac{v_2\rho_1}{4}\Bigg\{\sum_{\boldsymbol{k}} \frac{1}{E_{+,-} - E_{-,+} + \omega + i\delta}\left[1 + \frac{k^2(v_1^2 - v_2^2) - M_z^2}{E_{-,+}E_{+,+}}\right] + \sum_{\boldsymbol{k}} \frac{1}{E_{+,-} - E_{-,+} - \omega - i\delta}\left[1 + \frac{k^2(v_1^2 - v_2^2) - M_z^2}{E_{-,+}E_{+,+}}\right]\Bigg\} \tag{S.60}$$

$$= \frac{v_2\rho_1}{4}\Bigg\{\sum_{\boldsymbol{k}} \frac{1}{E_{+,+} + E_{-,+} - \omega - i\delta}\left[1 + \frac{k^2(v_1^2 - v_2^2) - M_z^2}{E_{-,+}E_{+,+}}\right] + \sum_{\boldsymbol{k}} \frac{1}{E_{+,+} + E_{-,+} + \omega + i\delta}\left[1 + \frac{k^2(v_1^2 - v_2^2) - M_z^2}{E_{-,+}E_{+,+}}\right]\Bigg\} \tag{S.61}$$

$$= \frac{v_2\rho_1}{4}\Bigg\{\sum_{\boldsymbol{k}} i\pi\delta(E_{+,+}(\boldsymbol{k}) + E_{-,+}(\boldsymbol{k}) - \omega)\left[1 + \frac{k^2(v_1^2 - v_2^2) - M_z^2}{E_{-,+}E_{+,+}}\right] + \mathcal{P}\sum_{\boldsymbol{k},\tau} \frac{1}{E_{+,+} + E_{-,+} - \tau\omega}\left[1 + \frac{k^2(v_1^2 - v_2^2) - M_z^2}{E_{-,+}E_{+,+}}\right]\Bigg\}, \tag{S.62}$$

where we assume $\omega > 0$. Here we first consider the first term $(A_1)$. We define $x(k) \equiv E_{+,+}(k) + E_{-,+}(k) = \sqrt{M_z^2 + k^2(v_1+v_2)^2} + \sqrt{M_z^2 + k^2(v_1-v_2)^2}$, then,

$$(A_1) = \frac{iv_2\rho_1}{8}\int_{2|M_z|}^{x(k_c)} dx\ \delta(x-\omega)\left[\frac{\sqrt{M_z^2 + k^2(v_1+v_2)^2}\sqrt{M_z^2 + k^2(v_1-v_2)^2}}{(v_1+v_2)^2\sqrt{M_z^2 + k^2(v_1-v_2)^2} + (v_1-v_2)^2\sqrt{M_z^2 + k^2(v_1+v_2)^2}}\right] \times\left[1 + \frac{k^2(v_1^2 - v_2^2) - M_z^2}{\sqrt{M_z^2 + k^2(v_1+v_2)^2}\sqrt{M_z^2 + k^2(v_1-v_2)^2}}\right],\quad k = \sqrt{\frac{(v_1^2+v_2^2)x^2 + \sqrt{16M_z^2v_1^2v_2^2x^2 + (v_1^2-v_2^2)^2x^4}}{8v_1^2v_2^2}}. \tag{S.63}$$

Finally, we get

$$(A_1) = \frac{iv_2\rho_1}{8}\Theta(\omega - 2|M_z|)\Theta(x(k_c) - \omega)\left[\frac{\sqrt{M_z^2 + k^2(v_1+v_2)^2}\sqrt{M_z^2 + k^2(v_1-v_2)^2}}{(v_1+v_2)^2\sqrt{M_z^2 + k^2(v_1-v_2)^2} + (v_1-v_2)^2\sqrt{M_z^2 + k^2(v_1+v_2)^2}}\right] \times\left[1 + \frac{k^2(v_1^2 - v_2^2) - M_z^2}{\sqrt{M_z^2 + k^2(v_1+v_2)^2}\sqrt{M_z^2 + k^2(v_1-v_2)^2}}\right],\quad k = \sqrt{\frac{(v_1^2+v_2^2)\omega^2 + \sqrt{16M_z^2v_1^2v_2^2\omega^2 + (v_1^2-v_2^2)^2\omega^4}}{8v_1^2v_2^2}}. \tag{S.64}$$

In the range of $2|M_z| \ll \omega$ ($\ll x(k_c)$), one can obtain that $(A_1) \approx \lim_{M_z\to 0}(A_1) = \frac{i\rho_1}{16v_1}\omega$ for $v_1 > v_2 > 0$. Also, we consider the second term $(A_2)$:

$$(A_2) = \frac{v_2\rho_1}{4}\Bigg\{\mathcal{P}\sum_{\boldsymbol{k}} \frac{1}{E_{+,+} + E_{-,+} - \omega}\left[1 + \frac{k^2(v_1^2 - v_2^2) - M_z^2}{E_{-,+}E_{+,+}}\right] + \mathcal{P}\sum_{\boldsymbol{k}} \frac{1}{E_{+,+} + E_{-,+} + \omega}\left[1 + \frac{k^2(v_1^2 - v_2^2) - M_z^2}{E_{-,+}E_{+,+}}\right]\Bigg\}. \tag{S.65}$$

In the case of $\omega \ll 2|M_z|$, we expand $(A_2)$ as following:

$$(A_2) \approx \frac{v_2\rho_1}{8\pi}\int_0^{k_c} dk \frac{2k\left[1 + \frac{k^2(v_1^2-v_2^2)-M_z^2}{\sqrt{M_z^2+k^2(v_1+v_2)^2}\sqrt{M_z^2+k^2(v_1-v_2)^2}}\right]}{\sqrt{M_z^2 + k^2(v_1+v_2)^2} + \sqrt{M_z^2 + k^2(v_1-v_2)^2}} + \frac{2k\left[1 + \frac{k^2(v_1^2-v_2^2)-M_z^2}{\sqrt{M_z^2+k^2(v_1+v_2)^2}\sqrt{M_z^2+k^2(v_1-v_2)^2}}\right]\omega^2}{(\sqrt{M_z^2 + k^2(v_1+v_2)^2} + \sqrt{M_z^2 + k^2(v_1-v_2)^2})^3}$$

$$\approx \frac{v_2\rho_1}{8\pi}\left[\frac{2k_c}{v_1} - \frac{2M_z}{v_1^2 - v_2^2} + \frac{M_z\ln\left|\frac{v_1-v_2}{v_1+v_2}\right|}{2v_1v_2} + \frac{\omega^2}{16v_1^3v_2^3}\left(-2v_2\frac{M_z^2}{k_c^3} + \frac{v_1^2v_2 - 5v_2^3}{k_c} + \frac{2v_1v_2(3v_2^2 - v_1^2) - ((v_1^2+v_2^2)^2 - 4v_2^4)\ln\left|\frac{v_1-v_2}{v_1+v_2}\right|}{2M_z}\right)\right] \tag{S.66}$$

for $M_z > 0$ and $v_1 > v_2 > 0$. In the case of $2|M_z| \ll \omega \ll x(k_c)$, one can obtain that

$$(A_2) \approx \lim_{M_z\to 0}(A_2) = \frac{v_2\rho_1}{8\pi}\frac{2k_cv_1 - \frac{\omega}{2}\ln\left|\frac{1+\frac{2k_cv_1}{\omega}}{1-\frac{2k_cv_1}{\omega}}\right|}{v_1^2}. \tag{S.67}$$

In the case of $\omega \gg x(k_c)$, one can obtain that $(A_2) \propto \frac{1}{\omega^2}$.

### 2. $K_{12}(\omega)$

In the next, we calculate the first term of Eq. (S.53) and omit $\frac{1}{4}$ and $+i\delta$:

$$\begin{aligned}
&\sum_{n\in\text{occ},m\in\text{unocc}}\frac{\langle n|-v_2s_3\tau_1|m\rangle\langle m|\rho_2s_0\tau_2|n\rangle}{E_n-E_m+\omega}\\
&=-v_2\rho_2\Bigg[\frac{(\tau_1)_{11}\langle +-|s_3|++\rangle\langle ++|s_0|+-\rangle(\tau_2)_{11}}{E_{+,-}-E_{+,+}+\omega}+\frac{(\tau_1)_{12}\langle +-|s_3|-+\rangle\langle -+|s_0|+-\rangle(\tau_2)_{21}}{E_{+,-}-E_{-,+}+\omega}\\
&\qquad+\frac{(\tau_1)_{21}\langle --|s_3|++\rangle\langle ++|s_0|--\rangle(\tau_2)_{12}}{E_{-,-}-E_{+,+}+\omega}+\frac{(\tau_1)_{22}\langle --|s_3|-+\rangle\langle -+|s_0|--\rangle(\tau_2)_{22}}{E_{-,-}-E_{-,+}+\omega}\Bigg]\\
&=-v_2\rho_2\left[\frac{(\tau_1)_{12}\langle +-|s_3|-+\rangle\langle -+|s_0|+-\rangle(\tau_2)_{21}}{E_{+,-}-E_{-,+}+\omega}+\frac{(\tau_1)_{21}\langle --|s_3|++\rangle\langle ++|s_0|--\rangle(\tau_2)_{12}}{E_{-,-}-E_{+,+}+\omega}\right]\\
&=-iv_2\rho_2\left[\frac{\langle +-|s_3|-+\rangle\langle -+|s_0|+-\rangle}{E_{+,-}-E_{-,+}+\omega}-\frac{\langle --|s_3|++\rangle\langle ++|s_0|--\rangle}{E_{+,-}-E_{-,+}+\omega}\right],
\end{aligned} \tag{S.68}$$

where we use $E_{-,-}=-E_{-,+}, E_{+,+}=-E_{+,-}$. By using Eq. (S.55)–(S.57), we get

$$\begin{aligned}
&\sum_{n\in\text{occ},m\in\text{unocc}}\frac{\langle n|-v_2s_3\tau_1|m\rangle\langle m|\rho_2s_0\tau_2|n\rangle}{E_n-E_m+\omega}\\
&=-\frac{iv_2\rho_2}{E_{+,-}-E_{-,+}+\omega}\left[2\Big(\sin^2(\theta_+/2)\cos^2(\theta_-/2)-\sin^2(\theta_-/2)\cos^2(\theta_+/2)\Big)-i\sin(\phi_+-\phi_-)\sin(\theta_+)\sin(\theta_-)\right].
\end{aligned} \tag{S.69}$$

The second term is 0, then the response function is given by

$$\begin{aligned}
K_{12}(\omega)&=-\frac{iv_2\rho_2}{4}\left\{\sum_{\boldsymbol{k}}\frac{1}{E_{+,-}-E_{-,+}+\omega+i\delta}\left[\frac{M_z}{E_{-,+}}-\frac{M_z}{E_{+,+}}\right]-\sum_{\boldsymbol{k}}\frac{1}{E_{+,-}-E_{-,+}-\omega-i\delta}\left[\frac{M_z}{E_{-,+}}-\frac{M_z}{E_{+,+}}\right]\right\}\\
&=-\frac{iv_2\rho_2}{4}\left\{\sum_{\boldsymbol{k}}\frac{-1}{E_{+,+}+E_{-,+}-\omega-i\delta}\left[\frac{M_z}{E_{-,+}}-\frac{M_z}{E_{+,+}}\right]+\sum_{\boldsymbol{k}}\frac{1}{E_{+,+}+E_{-,+}+\omega+i\delta}\left[\frac{M_z}{E_{-,+}}-\frac{M_z}{E_{+,+}}\right]\right\}\\
&=-\frac{iv_2\rho_2}{4}\left\{\sum_{\boldsymbol{k}}-i\pi\delta(E_{+,+}(\boldsymbol{k})+E_{-,+}(\boldsymbol{k})-\omega)\left[\frac{M_z}{E_{-,+}}-\frac{M_z}{E_{+,+}}\right]\right.\\
&\qquad\left.+\mathcal{P}\sum_{\boldsymbol{k},\tau}\frac{\tau}{E_{+,+}+E_{-,+}+\tau\omega}\left[\frac{M_z}{E_{-,+}}-\frac{M_z}{E_{+,+}}\right]\right\},
\end{aligned} \tag{S.70}$$

where we assume $\omega > 0$. Here we first consider the first term $(B_1)$:

$$\begin{aligned}
(B_1)&=-\frac{v_2\rho_2M_z}{8}\int_{2|M_z|}^{x(k_c)}dx\;\delta(x-\omega)\left[\frac{\sqrt{M_z^2+k^2(v_1+v_2)^2}\sqrt{M_z^2+k^2(v_1-v_2)^2}}{(v_1+v_2)^2\sqrt{M_z^2+k^2(v_1-v_2)^2}+(v_1-v_2)^2\sqrt{M_z^2+k^2(v_1+v_2)^2}}\right]\\
&\quad\times\left[\frac{1}{\sqrt{M_z^2+k^2(v_1-v_2)^2}}-\frac{1}{\sqrt{M_z^2+k^2(v_1+v_2)^2}}\right],\quad k=\sqrt{\frac{(v_1^2+v_2^2)x^2+\sqrt{16M_z^2v_1^2v_2^2x^2+(v_1^2-v_2^2)^2x^4}}{8v_1^2v_2^2}}.
\end{aligned} \tag{S.71}$$

Finally, we get

$$(B_1) = -\frac{v_2\rho_2 M_z}{8}\Theta(\omega - 2|M_z|)\Theta(x(k_c)-\omega)\left[\frac{\sqrt{M_z^2+k^2(v_1+v_2)^2}\sqrt{M_z^2+k^2(v_1-v_2)^2}}{(v_1+v_2)^2\sqrt{M_z^2+k^2(v_1-v_2)^2}+(v_1-v_2)^2\sqrt{M_z^2+k^2(v_1+v_2)^2}}\right]$$
$$\times\left[\frac{1}{\sqrt{M_z^2+k^2(v_1-v_2)^2}}-\frac{1}{\sqrt{M_z^2+k^2(v_1+v_2)^2}}\right],\quad k=\sqrt{\frac{(v_1^2+v_2^2)\omega^2+\sqrt{16M_z^2v_1^2v_2^2\omega^2+(v_1^2-v_2^2)^2\omega^4}}{8v_1^2v_2^2}}. \tag{S.72}$$

In the range of $2|M_z| \ll \omega$ ($\ll x(k_c)$), one can obtain that $(B_1) \approx M_z \lim_{M_z\to 0}(B_1)/M_z = -\frac{v_2\rho_2 M_z}{8}\frac{v_2}{v_1^3-v_1v_2^2}$ for $v_1 > v_2 > 0$. Also, we consider the second term $(B_2)$:

$$(B_2) = -\frac{iv_2\rho_2}{4}\left\{\mathcal{P}\sum_{\boldsymbol{k}}\frac{-1}{E_{+,+}+E_{-,+}-\omega}\left[\frac{M_z}{E_{-,+}}-\frac{M_z}{E_{+,+}}\right]+\mathcal{P}\sum_{\boldsymbol{k}}\frac{1}{E_{+,+}+E_{-,+}+\omega}\left[\frac{M_z}{E_{-,+}}-\frac{M_z}{E_{+,+}}\right]\right\} \tag{S.73}$$

In the case of $\omega \ll 2|M_z|$, we expand $(B_2)$ as following:

$$(B_2) \approx \frac{iv_2\rho_2}{4\pi}\int_0^{k_c} dk\frac{k\left[\frac{M_z}{\sqrt{M_z^2+k^2(v_1-v_2)^2}}-\frac{M_z}{\sqrt{M_z^2+k^2(v_1+v_2)^2}}\right]}{(\sqrt{M_z^2+k^2(v_1+v_2)^2}+\sqrt{M_z^2+k^2(v_1-v_2)^2})^2}\omega$$
$$\approx \frac{iv_2\rho_2}{4\pi}\frac{-2v_1v_2+v^2\ln\left|\frac{v_1+v_2}{v_1-v_2}\right|}{8v_1^2v_2^2}\omega. \tag{S.74}$$

In the case of $2|M_z| \ll \omega \ll x(k_c)$, one can obtain that

$$(B_2) \approx M_z\lim_{M_z\to 0}(B_2)/M_z = -\frac{iv_2\rho_2 M_z}{8\pi}\frac{v_2\ln\left|\frac{1+\frac{2k_cv_1}{\omega}}{1-\frac{2k_cv_1}{\omega}}\right|}{v_1^3-v_1v_2^2}. \tag{S.75}$$

In the case of $\omega \gg x(k_c)$, one can obtain that $(B_2) \propto \frac{iM_z}{\omega}$.

---


[1] S. Kobayashi, Y. Yamazaki, A. Yamakage, and M. Sato, Majorana multipole response: General theory and application to wallpaper groups, Phys. Rev. B **103**, 224504 (2021).
[2] Y. Yamazaki, S. Kobayashi, and A. Yamakage, Electric Multipoles of Double Majorana Kramers Pairs, J. Phys. Soc. Jpn. **90**, 073701 (2021).
[3] A. Widera and H. Schäfer, Übergangsformen zwischen zintlphasen und echten salzen: Die verbindungen A3BO (MIT A = Ca, Sr, Ba und B = Sn, Pb), Mater. Res. Bull. **15**, 1805 (1980).
[4] J. Nuss, C. Mühle, K. Hayama, V. Abdolazimi, and H. Takagi, Tilting structures in inverse perovskites, M3TtO (M = Ca, Sr, Ba, Eu; Tt = Si, Ge, Sn, Pb), Acta Cryst. B **71**, 300 (2015).
[5] T. Kawakami, T. Okamura, S. Kobayashi, and M. Sato, Topological Crystalline Materials of $J = 3/2$ Electrons: Antiperovskites, Dirac Points, and High Winding Topological Superconductivity, Phys. Rev. X **8**, 041026 (2018).
[6] L. Elcoro, B. Bradlyn, Z. Wang, M. G. Vergniory, J. Cano, C. Felser, B. A. Bernevig, D. Orobengoa, G. de la Flor, and M. I. Aroyo, Double crystallographic groups and their representations on the Bilbao Crystallographic Server, J Appl. Cryst. **50**, 1457 (2017).
[7] Irreducible representations of SG $P4mm$ are referred from the database, which are compatible with those of WG $p4m$.
[8] T. Funato and M. Matsuo, Acoustic Rashba–Edelstein effect, J. Magn. Magn. Mater. **540**, 168436 (2021).
